# Supplementary material for: Shift current bulk photovoltaic effect influenced by quasiparticles and excitons
Source: arXiv:1811.05287 source file (2018-11-13)
Supplement: Supplementary file 1 [file supplement.pdf]

# Supplemental Material: Shift current bulk photovoltaic effect influenced by quasiparticles and excitons

Ruixiang Fei,[1] Liang Z. Tan,[2] and Andrew M. Rappe[1,*]

[1] Department of Chemistry, University of Pennsylvania, Philadelphia, Pennsylvania 19104-6323, USA
[2] Molecular Foundry, Lawrence Berkeley National Laboratory, Berkeley, California 94720, United States

## I. COMPUTATIONAL DETAILS

### A. GGA level and shift current

DFT calculations were conducted using a plane-wave basis with a 50 Ry energy cutoff with norm-conserving pseudopotentials for both $BaTiO_3$ and monolayer SnSe. For bulk $BaTiO_3$, an $8 \times 8 \times 8$ Monkhorst-Pack k grid for self-consistent evaluation of the charge densities. Monkhorst-Pack k grid of $24 \times 24 \times 24$, $48 \times 48 \times 48$ and $64 \times 64 \times 64$ are used to ensure a well-converged shift current response. For 2D SnSe, the structural relaxation self- consistent and non-self-consistent calculations, Monkhorst-Pack k grid of $12 \times 12 \times 1$, $48 \times 48 \times 1$ and $72 \times 72 \times 1$ are used to ensure a well-converged shift current response.

### B. Many body calculations

The static polarizability and the inverse dielectric matrix are calcluated using the static RPA polarizability using the following expression:

$$\chi_{GG'}(q,0) = \sum_{v}^{occ} \sum_{v}^{emp} \sum_{k} M^{*}_{cv}(k,q,G) M_{vc}(k,q,G') \frac{1}{E_v(k+q) - E_c(k)} \tag{S1}$$

where

$$M_{cv}(k,q,G) = \langle c, k+q | e^{i(q+G)\cdot r} | v, k \rangle \tag{S2}$$

are the plane-wave matrix elements. Here $q$ is a vector in the first Brillouin zone, $G$ is a reciprocal lattice vector.

For the GW calculation of intrinsic monolayer SnSe, to get a converged inverse dielectric matrix, the dielectric matrix is calculated on a $36 \times 36 \times 1$ with a summation of Nc=120 empty bands (Nv = 12 valence bands) and a cutoff of 8 Ry. The same number of bands are used in the summation of the self-energy with the static reminder approximation to accelerate convergence. A truncation to the Coulomb interaction is applied to eliminate interactions between periodic images. The BSE is solved on

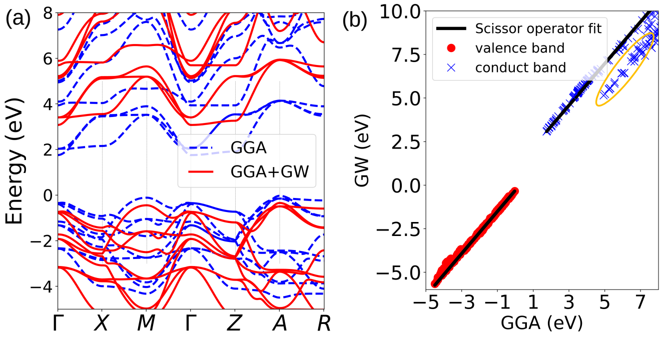


FIG. S1. The bandstructure of tetragonal phase $BaTiO_3$ at GGA level and *GW* level (a), The red solid line and blue dash line represent the band structure at the GW and GGA level, respectively. The energy difference between GGA and *GW* calculation (b), the red dot and blue cross dot represent the valence bands and conduction bands calculations, respectively, the black line is the scissor operator fit, and the yellow circle indicates the scissor approximation is invalid.

a finer $72 \times 72 \times 1$ k-grid. To get converged absorption for photon energy below 8 eV, 6 conduction bands and 9 valence bands are used for the BSE kernel and exciton absorption.

For the GW calculation of tetragonal $BaTiO_3$, the dielectric matrix is calculated on a $24 \times 24 \times 24$ with a summation of Nc=200 empty bands (Nv = 20 valence bands) and a cutoff of 8 Ry. The same number of bands are used in the summation of the self-energy with the static reminder approximation to accelerate convergence. The BSE is solved on a finer $48 \times 48 \times 48$ k-grid. To get converged absorption for photon energy below 10 eV, 9 conduction bands and 9 valence bands are used for the BSE kernel and exciton absorption calculation.

### C. Bandstructure and band width

In Fig S1a, we plot the GGA and GW band structure of BTO. The GW bandsture is not rigid shift of the GGA bands, as shown in Fig S1b. The slopes in Fig S1(b) shows the band widths are changed by the GW correction. The yellow circle in Fig S1(b) shows that the *GW* correction is not a uniform shift and rescaling, as there is a group of bands that does not fit to a scissors operator (starting from the fifth conduction band in S1a).

In Fig S2, the bandstructures at GGA and *GW* level and bandwiths changes are given. Compared with bulk

* rappe@sas.upenn.edu

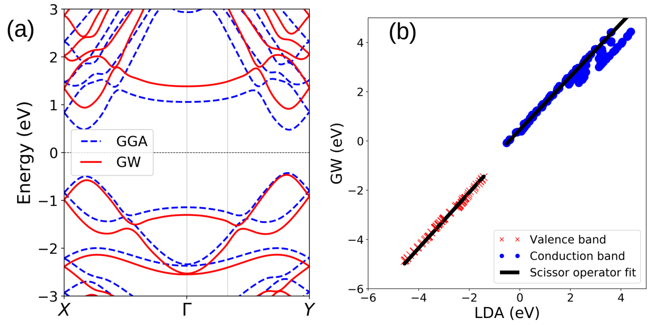


FIG. S2. The bandstructure of two dimensional SnSe at GGA level and $GW$ level (a), The red solid line and blue dash line represent the band structure at the $GW$ and GGA level, respectively. The energy difference between GGA and $GW$ calculation (b), the red cross dot and blue dot represent the valence bands and conduction bands calculations, respectively, the black line is the scissor operator fit, the slope represents the changes of bandwidths

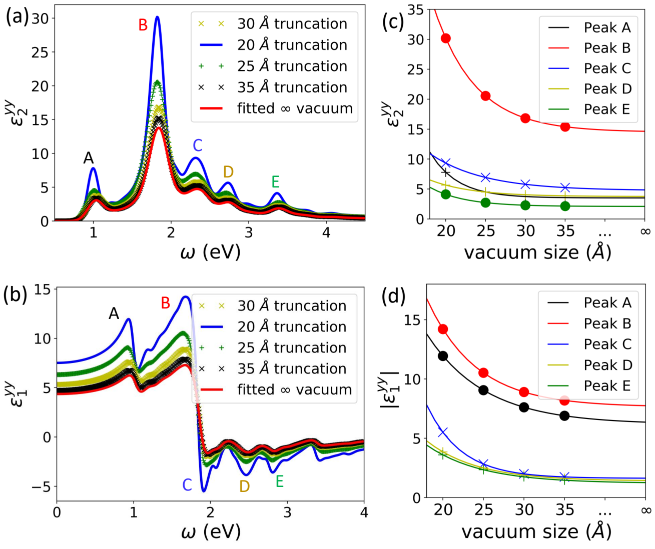


FIG. S3. The imaginary (a) and real part (b) of dielectric constant for two dimensional SnSe. The exponential decay fitting for the peaks of the imaginary (c) and real (d) part. 20, 25, 30, 35 Åvacuum are used to get the power law for the dielectric constant.

BTO, the bandwidths correction induced by $GW$ correction is smaller. Here, the $GW$ valence and conduction bandwidth increases by 13% and 8%, respectively.

### D. Dielectric constant for two dimensioanl

For two dimensional SnSe, the dielectric constant is strongly dependent on the supercell size. We found 20 Åof vacuum is not good enough for an accurate calculation of the dielectric constant. Here we use several supercell sizes, shown in Fig. S3, to extract the dielectric constant for SnSe. Fig S3 (c-d) shows the exponetial decay fitting for the main peaks of the imaginary and real parts of dielectric constant. Using these fitting parameters, we can extract the dielectric of SnSe with an infinite amount of vacuum. The value is very close to the dielectric constant calculated using 35 Åof vacuum.

## II. DERIVATIVE FOR CURRENT, ABSORPTION COEFFICIENT, REFLECTION RATIO

### A. Complex refraction index and dielectric constant

Using the simple relation between refraction index and complex dielectric constant

$$(a(\omega) + ib(\omega))^2 = \epsilon_1 + i\epsilon_2 \tag{S3}$$

one can get the complex refraction index by

$$\begin{aligned} a(\omega) &= \sqrt{\frac{1}{2}(\epsilon_1 + \sqrt{\epsilon_1^2 + \epsilon_2^2})} \\ b(\omega) &= \frac{\epsilon_2^2}{\sqrt{2(\epsilon_1 + \sqrt{\epsilon_1^2 + \epsilon_2^2})}} \end{aligned} \tag{S4}$$

where the $\epsilon_1(\omega)$ and $\epsilon_2(\omega)$ are the real and imaginary part of complex dielectric constant, respectively. Applying the linear response theory to the first order electric optical interaction[S1], the imaginary part $\epsilon_2(\omega)$ is calculated by [S2]

$$\epsilon_2(\omega)^{GGA} = \frac{16\pi e^2}{\omega^2} \sum_{c,v} |\langle v|\vec{v}|c\rangle|^2 \delta(\omega - (E_c - E_v)) \tag{S5}$$

where we set $\hbar = 1$, $\langle v|\vec{v}|c\rangle$ is velocity matrix between conduction band $|c\rangle$ and valence band $|v\rangle$ calculated from GGA approximation. When considering the quasiparticle correction

$$\langle v|\vec{v}|c\rangle^{GW} = \frac{E_c^{GW} - E_v^{GW}}{E_c^{GGA} - E_v^{GGA}} \langle v|\vec{v}|c\rangle^{GGA} \tag{S6}$$

The effect of this renormalization is that, taking into account the division by $\omega^2$, the weight of a transition is not changed when the transition is shifted to higher energies by the GW correction.

If considering the exciton effect in dielectric constant,

$$\epsilon_2(\omega)^{GGA} = \frac{16\pi e^2}{\omega^2} \sum_{S} |\langle 0|\vec{v}|S\rangle|^2 \delta(\omega - (\Omega_S)) \tag{S7}$$

where the correlated e-h excitation $S$ of energy $\Omega^S$ is expanded on the basis of e-h pairs $|S\rangle = \sum A^S_{vc\mathbf{k}} |vc\mathbf{k}\rangle$. Next using the simple Kramers-Krönig relation, the real part $\epsilon_1(\omega)$ is

$$\epsilon_1(\omega) = 1 + \frac{2}{\pi} p \int_0^\infty d\omega' \frac{\omega' \epsilon_2(\omega)}{\omega'^2 - \omega^2} \tag{S8}$$

### B. Absorption coefficient

Considering a monochromatic electromagnetic wave propagate in material,

$$E_y = E_0 e^{i\omega(\frac{n(\omega)}{c}z-t)} = E_0 e^{i\omega(\frac{a(\omega)+ib(\omega)}{c}z-t)} \\ = E_0 e^{-\frac{-b(\omega)\omega}{c}z} e^{i\omega(\frac{a(\omega)\omega}{c}z-t)} \tag{S9}$$

where c is speed of light, $n(\omega) = a(\omega) + ib(\omega)$ is the complex refraction index. Since the light intensity is proportional to $E^2$, the intensity decay as a factor $e^{-\frac{2\omega b(\omega)}{c}z}$, thus the absorption coefficient $\alpha(\omega)$ is

$$\alpha(\omega) = \frac{2\omega b(\omega)}{c} = \frac{\omega\epsilon_2(\omega)}{a(\omega)c} \\ = \frac{\omega}{c}\sqrt{2}\sqrt{\sqrt{\epsilon_1^2(\omega)+\epsilon_2^2(\omega)} - \epsilon_1(\omega)} \tag{S10}$$

### C. Reflection coefficient and Reflection ratio

The normal incidence reflectivity (reflection ratio) $R$ is written as [S3]

$$R = |\frac{E_{ref}}{E_{in}}|^2 = |\frac{1-n(\omega)}{1+n(\omega)}|^2 \\ = \frac{(a(\omega)-1)^2 + b(\omega)^2}{(a(\omega)+1)^2 + b(\omega)^2} \tag{S11}$$

and the relflection coefficient for the wave itself is given by

$$r = \frac{1-a(\omega)-ib(\omega)}{1+a(\omega)+ib(\omega)} \tag{S12}$$

where the reflectivity (or reflection ratio) $R$ is a number less than unity and $r$ has an amplitude of less than unity. We have now related one of the physical observables to the optical constants. To relate these results to the power absorbed and transmitted at normal incidence, we utilize the following relation which expresses the idea that all the incident power is either reflected, absorbed, or transmitted

$$1 = R + A + T \tag{S13}$$

where $R$, $A$, and $T$ are the fraction of the power that is reflected, absorbed, and transmitted, respectively.

### D. shift current for bulk and two dimensional materials

For a material with d thickness, the shift current is

$$J_{ssQ}(\omega)\cdot d\cdot w = \int_0^d K_{ssQ}(1-R)e^{-\alpha_{ss}(\omega)z}\cdot dz\cdot w\cdot I_Q \\ = \frac{K_{ssQ}}{\alpha_{ss}(\omega)}(1-R_{ss})(1-e^{-\alpha_{ss}(\omega)d})\cdot w\cdot I_s^2 \tag{S14}$$

For bulk crystal e.g. $BaTiO_3$, the depth $d$ is much larger than length scale of inverse absorption coefficient $\alpha_{ss}^{-1}$ (hundreds $\mu m$), the total current is

$$J_{ssQ} = \frac{\sigma_{ssQ}}{\alpha_{ss}(\omega)}(1-R_{ss})\cdot w\cdot E_s^2 = G_{ssQ}(1-R_{ss})\cdot w\cdot I_s \tag{S15}$$

where $G_{ssQ}$ is the Glass coefficient [S4]. For very 2D material, e.g. 2D SnSe, the total current is

$$J_{ssQ} = \sigma_{ssQ}d(1-R_{ss})wE_s^2 = K_{ssQ}d(1-R_{ss})\cdot w\cdot I_s \tag{S16}$$


[S1] G. Giuliani and G. Vignale, *Quantum theory of the electron liquid* (Cambridge university press, 2005).

[S2] M. Rohlfing and S. G. Louie, Phys. Rev. B **62**, 4927 (2000).

[S3] M. Dresselhaus, G. Dresselhaus, S. Cronin, and A. Filho, *Solid State Properties: From Bulk to Nano*, Graduate Texts in Physics (Springer Berlin Heidelberg, 2018).

[S4] A. Glass, D. Von Der Linde, T. Negran, A. M. Glass, D. von der Linde, and T. J. Negran, .
